# Supplementary material for: A Hybrid Discrete Exterior Calculus Discretization and Fourier Transform of the Incompressible Navier-Stokes Equations in 3D
Source: arXiv:2409.04731 source file (2024-09-07)
Supplement: Supplementary file 1 [file Appendix_A.tex]

% Appendix A File

\refstepcounter{chapter}%
\chapter*{\thechapter \quad Appendix A Title}
\label{appendixA}

Detailed experimental procedures, data tables, computer programs, etc. may be placed in appendices. This may be particularly appropriate if the dissertation or thesis includes several published papers.
