# Supplementary material for: A Hybrid Discrete Exterior Calculus Discretization and Fourier Transform of the Incompressible Navier-Stokes Equations in 3D
Source: arXiv:2409.04731 source file (2024-09-07)
Supplement: Supplementary file 2 [file Appendix_B.tex]

% Appendix B File

\refstepcounter{chapter}%
\chapter*{\thechapter \quad Appendix B Title}
\label{appendixB}

Your content goes here.
